# Supplementary material for: Stable algorithms for general linear systems by preconditioning the normal equations
Source: arXiv:2502.17767 source file (2025-03-04)
Supplement: Supplementary file 1 [file siam_supplement.tex]

% SIAM Supplemental File Template
\documentclass[review,supplement,hidelinks,onefignum,onetabnum,backref]{siamart220329}

\input{siam_shared}

\externaldocument[][nocite]{siam_article}

% Optional PDF information
\ifpdf
\hypersetup{
  pdftitle={Supplementary Materials: },
  pdfauthor={E. N. Epperly}
}
\fi

\begin{document}

\maketitle

\input{../general/supplement}

\bibliographystyle{siamplain}
\bibliography{../general/refs}

\end{document}
